# Supplementary material for: Resonant-light diffusion in a disordered atomic layer
Source: arXiv:1802.04018 ancillary file (2018-06-18)
Supplement: Supplementary file 1 [file supmat.pdf]

# Supplemental Materials for: Resonant-light diffusion in a disordered atomic layer

## I. IMAGING SYSTEM CALIBRATION

The fluorescence light emitted by the atomic cloud is collected using a microscope objective with a numerical aperture of 0.4. Using the full aperture of this objective leads to a deterioration of the sharpness of the decay signals we measure. We attribute this effect to residual optical aberrations which are important for photons propagating at large angle with respect to the optical axis. These aberrations can be due to the optics we used or to an imperfect alignment of these optics. To limit the effective aperture we use an iris (see Fig. 1c in the main text). We have empirically adjusted its opening to get the sharpest decay while not decreasing too much the detected signal. We report in Supplementary Fig. 1 the decay length and the signal measured for the atomic fluorescence and for the excitation light beam as a function of the opening of this iris. The atomic fluorescence signal is obtained for the densest cloud excited on resonance.

First, we consider the profile of the excitation light beam on the camera. This is still done by detecting the polarization perpendicular to the excitation light beam polarization but with unblocking the residual transmitted light, which originates from the non-perfect polarization components. Because of the finite optical resolution, the edges of the beam profile are not perfectly sharp. We apply the same procedure as for the fluorescence signal to determine an effective decay length from an exponential fit. We observe that the decay length and the signal amplitude are almost independent of this opening, as expected for a collimated beam impinging on the atoms which is thus not affected by the spatial filtering. It also shows that our optical system allows to measure decay lengths below $1\,\mu$m. Second, we consider the atomic fluorescence. The decay length which increases for large opening is almost constant for small openings ($4 < D_{\rm iris} < 7$ mm). The number of collected photons increases monotonically with the iris diameter. We have chosen for the data presented in the main text an opening of $D_{\rm iris} = 6.5$ mm, inside the region where $\xi$ is rather constant but maximizing the measured signal.

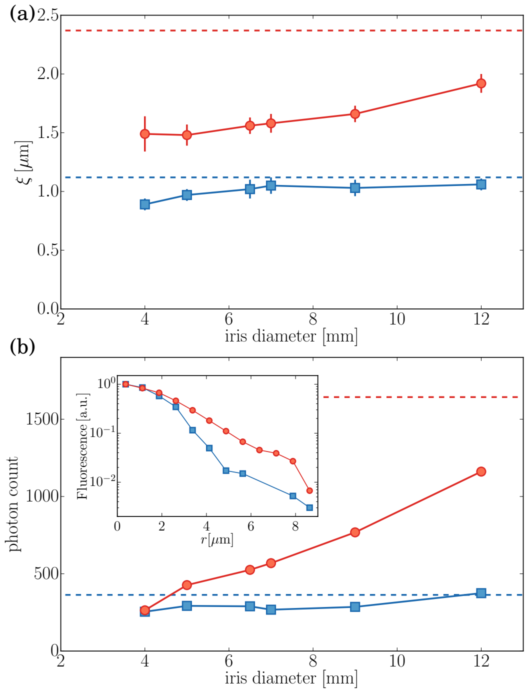


Supplementary Fig. 1 . Influence of the filtering iris. Measured decay length (a) and total number of photons detected on the CCD camera (b) for the light excitation beam alone (squares) and for the atomic fluorescence (disks). For both graphs, the dashed lines are the corresponding results without the iris. Vertical error bars correspond to the standard deviation of the results of exponential fits to the data obtained with a bootstrap approach. Each data set is obtained from the average of 50 measurements. The inset in (b) shows the fluorescence and excitation light beam signals (both normalized to unity) for $D_{\rm iris} = 6.5$ mm.

## II. THEORY

We detail here the derivation of the semi-analytical model of the main text. First, we recall that at any detuning, the decay length is given by

$$k\xi = \frac{k\ell}{\sqrt{1-\cos\theta_0}}, \qquad (1)$$

where the variation of the maximum emission angle $\theta_0$ with $\Delta$ is depicted in the insets of Fig. 4(a) in the main text. When $\Delta = 0$, we have $\tan\theta_0 = \ell/\sqrt{\sigma/\pi}$, which straightforwardly leads to Eq.(3) of the main text. When $\Delta \neq 0$, the geometry of the cone is modified by the changes of $\ell$ and $\sigma$ with detuning, which are symmetric with respect to $\Delta = 0$. But, in addition, the photon trajectories are bent and $\theta_0$ has to be determined by taking into account the curvatures of these trajectories.

To estimate it, we use the parametrization shown in Supplementary Fig. 3 (here displayed for $\Delta < 0$). The $z$ axis is normal to the atomic layer, with $z = 0$ corresponding to the center of the layer where the density is maximum. From the figure we have $\sin\theta = dr/\sqrt{dr^2+dz^2} = 1/\sqrt{1+(dz/dr)^2}$. Using that $\sin\theta = \sin\theta_0\, n(z=0)/n(z)$ (Snell's law), we infer

$$\left(\frac{dz}{dr}\right)^2 = \left[\frac{n(z)}{n_0\sin\theta_0}\right]^2 - 1, \qquad (2)$$

where $n_0 = n(z=0)$. To solve Eq. (2), we use a low-density approximation for the refractive-index profile of the layer:

$$n(z) \simeq 1 - \frac{3\pi\rho_{3D}(z)}{k^3}\frac{\delta}{1+\delta^2}, \qquad (3)$$

where $\delta = 2\Delta/\Gamma$ and $\rho_{3D}(z)$ is the density profile of the cloud. Note that the change of the index of refraction is maximal for

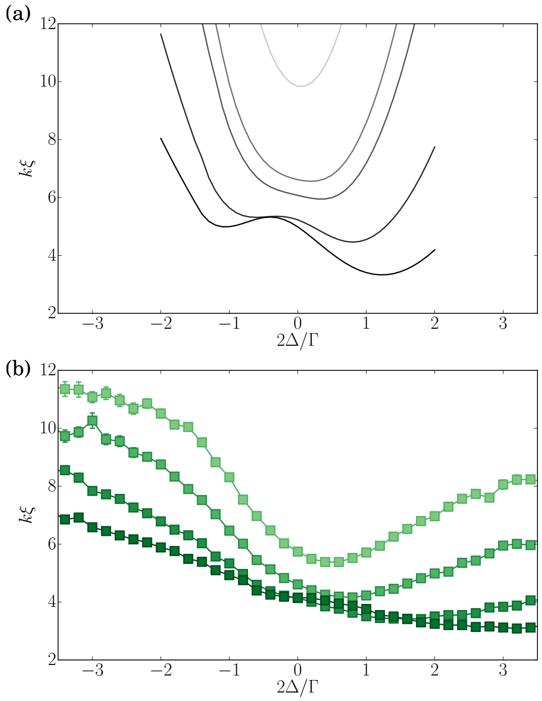


Supplementary Fig. 2 . Role of the detuning. (a) Results from the coupled dipole model with $\rho_{3D}k^{-3}$=0.01, 0.02, 0.05, and 0.1 (from top to bottom) and with, for all curves, $k\Delta z$ = 0.3. Error bars, which are mostly smaller than the size of the points, represent the statistical error obtained from the fitting procedure. (b) Results from the analytical model with $\rho_{3D}k^{-3}$=0.01, 0.02, 0.025, 0.05 and 0.1 (from top to bottom).

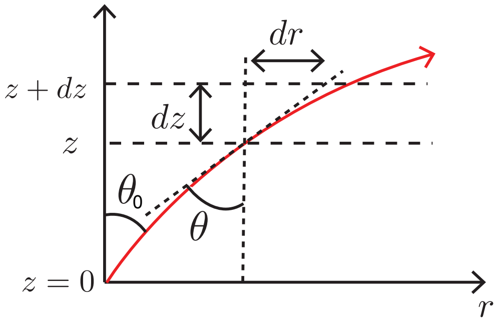


Supplementary Fig. 3 . Parametrization of a photon trajectory.

$\delta = 1$ and this formula thus holds for $\rho_{3D}k^{-3} < 2/(3\pi)$. To make the calculation analytical, we approximate the density profile by a parabolic one such that $n(z = 0) = n_0 = 1 - (3\pi\rho_{3D}\delta)/[k^3(1+\delta^2)]$ and $n(z = \sqrt{\sigma/\pi}) = 1$:

$$n(z) \simeq n_0 - \frac{n_0 - 1}{\sigma/\pi} z^2. \quad (4)$$

Inserting this profile into Eq. (2), we find the differential equation for the photon trajectory:

$$\frac{d^2 z}{dr^2} + \frac{2(n_0-1)z}{n_0(\sigma/\pi)\sin^2\theta_0} - \left(\frac{n_0-1}{n_0}\right)^2 \frac{2z^3}{(\sigma/\pi)^2\sin^4\theta_0} = 0, \quad (5)$$

whose solution is given by

$$z(r) = \frac{\sqrt{\sigma/\pi}\cos^2\theta_0}{\sqrt{n_0-1}} \frac{1}{1-\mathrm{sg}(\Delta)\sin\theta_0} \frac{1}{\sqrt{1+\mathrm{sg}(\Delta)\sin\theta_0}}$$

$$\times \mathrm{sn}\left[\frac{r\sqrt{n_0-1}}{\sqrt{\sigma/\pi}\sin\theta_0}\sqrt{1-\mathrm{sg}(\Delta)\sin\theta_0}, \frac{1+\mathrm{sg}(\Delta)\sin\theta_0}{1-\mathrm{sg}(\Delta)\sin\theta_0}\right], \quad (6)$$

where sn is the sinus Jacobi elliptic function, sg the sign function and $n_0 = n(z=0) = 1 - (3\pi\rho_{3D}\delta)/[k^3(1+4\Delta^2/\Gamma^2)]$. The angle $\theta_0$ is finally obtained from the implicit equation

$$z(r = \ell) = \sqrt{\sigma/\pi}. \quad (7)$$

For positive detuning, Eq. (7) always has a solution for $\theta$. At large detuning, this solution approaches $\pi/2$, a regime where $k\xi(\delta \gg 1) \simeq k\ell$ (note that this asymptotic result coincides with the prediction of Eq. (3) of the main text at large detuning). For negative detuning on the other hand, Eq. (7) has no solution when $\delta$ is smaller than a certain $\delta_c$, which is due to the phenomenon of total reflection. When $\delta < \delta_c$, the escape probability $p$ is no longer limited by the presence of the surrounding scatterers but by the bending of trajectories. In this regime, the radius of the escape cylinder is thus no longer given by $\ell$, but by the length $\ell_c$ where $dz/dr(r = \ell_c) = 0$ ($\ell_c$ coinciding with $\ell$ exactly at $\delta = \delta_c$). Consequently, when $\delta < \delta_c$ the angle $\theta$ is a solution of the implicit equation

$$z(\ell_c) = \sqrt{\sigma/\pi} \text{ with } \frac{dz}{dr}(r = \ell_c) = 0. \quad (8)$$

The curves shown in Supplementary Fig. 2(a) and in the main text are obtained by numerically solving Eq. (7) (for $\delta > \delta_c$) and Eq. (8) (for $\delta < \delta_c$) for $\theta_0$, then computing $k\xi$ using Eq. (1). The asymmetry of the decay length with detuning is more pronounced at low densities for the coupled dipole model than for the guiding model. This indicates that our simple guiding model gives a good qualitative picture but, in addition, cooperative effects plays a substantial role in our experiments. One could take into account, at first order, these cooperative effects by a suitable modification of the cross section and linewidth appearing in Eq. (1). Finally, we show in Supplementary Fig. 2(b) complementary results of the coupled dipole simulations for additional values of the atomic density and a constant thickness. For all densities we observe a similar asymmetry as in Fig. 4b in the main text. When increasing density, the resonance peak gets broader, as observed in transmission experiments [**?** ]. Note that the density $\rho k^{-3} = 0.1$ is the highest value we could reach in our simulations and remains lower than the achieved experimental densities.

[] L. Corman, J. L. Ville, R. Saint-Jalm, M. Aidelsburger, T. Bienaimé, S. Nascimbène, J. Dalibard, and J. Beugnon, Phys. Rev. A **96**, 053629 (2017).
